# Supplementary material for: Estimating the number of zeros of Dedekind zeta-functions
Source: arXiv:2510.27444 ancillary file (2026-10-12)
Supplement: Supplementary file 1 [file mathematica_documentation.pdf]

## Lemma 2.1

The following computes the zeroes of the derivative of  $h(t)$ .

(Debug) In[1]:=

```
H[t_, a1_, a2_, a3_, d_] := 2 ArcTan[(d + 0.5)/t] + 2 ArcTan[(d - 0.5)/t] - ArcTan[(2 d + 0.5)/t] -
ArcTan[(2 d - 0.5)/t] - Pi/4 (d * a1 * ((d + 0.5)/((d + 0.5)^2 + t^2) + (d - 0.5)/((d - 0.5)^2 + t^2)) +
d^2 a2 * ((d + 0.5)^2 - t^2)/((d + 0.5)^2 + t^2)^2 + ((d - 0.5)^2 - t^2)/((d - 0.5)^2 + t^2)^2) +
a3 * (2 (d + 0.5) t/((d + 0.5)^2 + t^2)^2 + 2 (d - 0.5) t/((d - 0.5)^2 + t^2)^2))
FunctionRange[H[x, 1.07, 0.93, 0.365, 0.722], x, y]
```

(Debug) Out[2]:=

-14.352 < y < 0.

(Debug) In[5]:=

```
H1[d_, a1_, a2_, a3_, t_] := (2 d + 1/2)/((2 d + 1/2)^2 + t^2) +
(2 d - 1/2)/((2 d - 1/2)^2 + t^2) - (2 d + 1)/((d + 1/2)^2 + t^2) - (2 d - 1)/((d - 1/2)^2 + t^2) +
Pi/4 (d a1 (((2 d + 1) t)/((d + 1/2)^2 + t^2)^2 + ((2 d - 1) t)/((d - 1/2)^2 + t^2)^2) +
d^2 a2 ((2 t (3 (d + 1/2)^2 - t^2))/((d + 1/2)^2 + t^2)^3 +
(2 t (3 (d - 1/2)^2 - t^2))/((d - 1/2)^2 + t^2)^3) - a3 ((2 (d + 1/2) (d + 1/2)^2 - 3 t^2))/
((d + 1/2)^2 + t^2)^3 + (2 (d - 1/2) (d - 1/2)^2 - 3 t^2))/((d - 1/2)^2 + t^2)^3);
NSolve[{H1[0.722, 1.07, 0.93, 0.365, t], -Infinity < t < Infinity}, t]
```

(Debug) Out[6]:=

```
{{t -> -0.791179}, {t -> -0.345961}, {t -> 0.0520308},
{t -> 0.90911}, {t -> 1.33512}, {t -> 2.74995}, {t -> 5.86346}}
```

Evaluating the function  $h(t)$  at these extrema yields:

(Debug) In[7]:=

```
H[t_, a1_, a2_, a3_, d_] := 2 ArcTan[(d + 0.5)/t] + 2 ArcTan[(d - 0.5)/t] - ArcTan[(2 d + 0.5)/t] -
ArcTan[(2 d - 0.5)/t] - Pi/4 (d * a1 * ((d + 0.5)/((d + 0.5)^2 + t^2) + (d - 0.5)/((d - 0.5)^2 + t^2)) +
d^2 a2 * ((d + 0.5)^2 - t^2)/((d + 0.5)^2 + t^2)^2 + ((d - 0.5)^2 - t^2)/((d - 0.5)^2 + t^2)^2) +
a3 * (2 (d + 0.5) t/((d + 0.5)^2 + t^2)^2 + 2 (d - 0.5) t/((d - 0.5)^2 + t^2)^2));
H[-0.791179, 1.07, 0.93, 0.365, 0.722]
```

(Debug) Out[8]:=

-0.279058

(Debug) In[9]:=

```
H[-0.345961, 1.07, 0.93, 0.365, 0.722]
```

(Debug) Out[9]:=

-0.0001916

(Debug) In[10]:=

```
H[0.0520308, 1.07, 0.93, 0.365, 0.722]
```

(Debug) Out[10]:=

-9.68924

```
(Debug) In[11]:=
H[0.90911, 1.07, 0.93, 0.365, 0.722]
```

```
(Debug) Out[11]=
-0.000224576
```

```
(Debug) In[12]:=
H[1.33512, 1.07, 0.93, 0.365, 0.722]
```

```
(Debug) Out[12]=
-0.00326464
```

```
(Debug) In[13]:=
H[2.74995, 1.07, 0.93, 0.365, 0.722]
```

```
(Debug) Out[13]=
-0.000152467
```

```
(Debug) In[14]:=
H[5.86346, 1.07, 0.93, 0.365, 0.722]
```

```
(Debug) Out[14]=
-0.0007888
```

Lemma 2.3. We need to verify the range of the functions  $E_u(s(s-1))(T,d)$  and  $E_l(s(s-1))(T,d)$ , which we denote by  $E_1$  and  $E_2$  respectively. We can see that  $E_1(t)$  is increasing for  $t \geq 1$  and  $E_2$  is decreasing for  $t \geq 1$ .

```
(Debug) In[15]:=
E1[t_, d_, a1_, a2_, a3_] :=
4 / Pi (ArcTan[t / (d + 1/2)] + ArcTan[t / (d - 1/2)]) - 2 / Pi (ArcTan[t / (2 d + 1/2)] + ArcTan[t / (2 d - 1/2)]) +
d * a1 / 2 ((d + 1/2) / ((d + 1/2)^2 + t^2) + (d - 1/2) / ((d - 1/2)^2 + t^2)) -
d^2 a2 / 2 (((d + 1/2)^2 - t^2) / ((d + 1/2)^2 + t^2)^2 + ((d - 1/2)^2 - t^2) / ((d - 1/2)^2 + t^2)^2) +
a3 / 2 (2 (d + 1/2) t / ((d + 1/2)^2 + t^2)^2 + 2 (d - 1/2) t / ((d - 1/2)^2 + t^2)^2);
FunctionMonotonicity[{E1[x, 0.722, 1.07, 0.93, 0.365], x >= 1}, x]
```

```
(Debug) Out[16]=
-1
```

```
(Debug) In[17]:=
E2[t_, d_, a1_, a2_, a3_] :=
4 / Pi (ArcTan[t / (d + 1/2)] + ArcTan[t / (d - 1/2)]) - 2 / Pi (ArcTan[t / (2 d + 1/2)] + ArcTan[t / (2 d - 1/2)]) -
d * a1 / 2 ((d + 1/2) / ((d + 1/2)^2 + t^2) + (d - 1/2) / ((d - 1/2)^2 + t^2)) +
d^2 a2 / 2 (((d + 1/2)^2 - t^2) / ((d + 1/2)^2 + t^2)^2 + ((d - 1/2)^2 - t^2) / ((d - 1/2)^2 + t^2)^2) +
a3 / 2 (2 (d + 1/2) t / ((d + 1/2)^2 + t^2)^2 + 2 (d - 1/2) t / ((d - 1/2)^2 + t^2)^2);
FunctionMonotonicity[{E2[x, 0.722, 1.07, 0.93, 0.365], x >= 1}, x]
```

```
(Debug) Out[18]=
1
```

From this we obtain the range of these functions for  $t \geq 1$  by evaluating  $E_1(1)$  and  $E_2(1)$  because both  $E_1(t)$  and  $E_2(t)$  approach 2 as  $t$  goes to infinity.

(Debug) In[19]:=

**E1[1, 0.722, 1.07, 0.93, 0.365]**

(Debug) Out[19]=

2.38073

(Debug) In[20]:=

**E2[1, 0.722, 1.07, 0.93, 0.365]**

(Debug) Out[20]=

1.4585

Corollary 2.5. We need to verify the estimates for the third derivatives of  $f(x)$ ,  $g(x)$ , and  $h(x)$ . We denote these by  $f_3$ ,  $g_3$ , and  $h_3$  respectively.

(Debug) In[21]:=

**f3[x\_] := -3 / x ^ 4 + 24 / x ^ 5 - 6 / (x ^ 4 (Exp[x] - 1)) - 6 Exp[x] / (x ^ 3 (Exp[x] - 1) ^ 2) -  
 3 Exp[x] (Exp[x] + 1) / (x ^ 2 (Exp[x] - 1) ^ 3) - Exp[x] (Exp[2 x] + 4 Exp[x] + 1) / (x (Exp[x] - 1) ^ 4);**  
**N[FunctionRange[{f3[x], x ≥ 0}, x, y]]**

(Debug) Out[22]=

 $-0.0000702347 \leq y \leq 0.000978005$ 

(Debug) In[23]:=

**g3[x\_] := 6 / x ^ 4 - Exp[x] (Exp[2 x] + 4 Exp[x] + 1) / (Exp[x] - 1) ^ 4;**  
**N[FunctionRange[{g3[x], x ≥ 0}, x, y]]**

(Debug) Out[24]=

 $-0.00833333 < y \leq 0.00251824$ 

(Debug) In[25]:=

**h3[x\_] := 3 Exp[x] (Exp[x] + 1) / (Exp[x] - 1) ^ 3 - x Exp[x] (Exp[2 x] + 4 Exp[x] + 1) / (Exp[x] - 1) ^ 4;**  
**N[FunctionRange[{h3[x], x ≥ 0}, x, y]]**

(Debug) Out[26]=

 $-0.0423706 \leq y < 0.$ 

Lemma 2.6. Estimates for  $U_{\{1,1\}}(T)$  and  $UB_1(T)$ , which we denote by  $U11$  and  $UB1$  respectively:

(Debug) In[27]:=

**U11[d\_, a1\_, a2\_, a3\_, t\_] := (t / Pi) Log[1 + ((1 + 2 d) / (2 t)) ^ 2] - (t / (2 Pi)) Log[1 + ((1 + 4 d) / (2 t)) ^ 2] +  
 (d a1 / 8) Log[1 + ((1 + 2 d) / (2 t)) ^ 2] + ((2 d - 1) / Pi) ArcTan[t / (d + 1 / 2)] -  
 ((4 d - 1) / (2 Pi)) ArcTan[t / (2 d + 1 / 2)] - (2 t) / (3 Pi ((d + 1 / 2) ^ 2 + t ^ 2)) + t / (3 Pi ((2 d + 1 / 2) ^ 2 + t ^ 2)) -  
 (d a1 / 4) ((d + 1 / 2) / ((d + 1 / 2) ^ 2 + t ^ 2) + ((d + 1 / 2) ^ 2 - t ^ 2) / (3 ((d + 1 / 2) ^ 2 + t ^ 2) ^ 2)) +  
 (d ^ 2 a2 / 4) ((d + 1 / 2) / ((d + 1 / 2) ^ 2 + t ^ 2) + ((d + 1 / 2) ^ 2 - t ^ 2) / (((d + 1 / 2) ^ 2 + t ^ 2) ^ 2)) +  
 (a3 / 4) (t / ((d + 1 / 2) ^ 2 + t ^ 2) - (2 (d + 1 / 2) t) / (((d + 1 / 2) ^ 2 + t ^ 2) ^ 2));**  
**UB1[d\_, a1\_, a2\_, a3\_, t\_] := (4 / Pi) (1 / 360 + 1 / (1022 (d + 1 / 2))) / ((d + 1 / 2) ^ 2 + t ^ 2) ^ (3 / 2) +  
 (2 / Pi) (1 / 360 + 1 / (1022 (d + 1 / 4))) / ((d + 1 / 4) ^ 2 + (t / 2) ^ 2) ^ (3 / 2) +  
 (d a1 / 4) / (120 ((d / 2 + 1 / 4) ^ 2 + (t / 2) ^ 2) ^ (3 / 2)) +  
 (d ^ 2 a2 / 8 + a3 / 8) (1 / 6 + 1 / (23 (d / 2 + 1 / 4))) / ((d / 2 + 1 / 4) ^ 2 + (t / 2) ^ 2) ^ (3 / 2);**  
**FunctionRange[{U11[0.722, 1.07, 0.93, 0.365, x] + UB1[0.722, 1.07, 0.93, 0.365, x], x ≥ 1}, x, y]**

(Debug) Out[29]=

 $-0.25 < y \leq 0.0489105$

Estimates for  $L_{\{1,1\}}(T)$  and  $LB_1(T)$ , which we denote by  $L11$  and  $LB1$  respectively:

(Debug) In[30]:=

$$\begin{aligned} L11[d_, a1_, a2_, a3_, t_] := & (t/Pi) \log[1 + ((1+2d)/(2t))^2] - (t/(2Pi)) \log[1 + ((1+4d)/(2t))^2] - \\ & (d a1/8) \log[1 + ((1+2d)/(2t))^2] + ((2d-1)/Pi) \operatorname{ArcTan}[t/(d+1/2)] - \\ & ((4d-1)/(2Pi)) \operatorname{ArcTan}[t/(2d+1/2)] - (2t)/(3Pi ((d+1/2)^2 + t^2)) + t/(3Pi ((2d+1/2)^2 + t^2)) + \\ & (d a1/4) ((d+1/2)/((d+1/2)^2 + t^2) + ((d+1/2)^2 - t^2)/(3((d+1/2)^2 + t^2)^2)) - \\ & (d^2 a2/4) ((d+1/2)/((d+1/2)^2 + t^2) + ((d+1/2)^2 - t^2)/(((d+1/2)^2 + t^2)^2)) + \\ & (a3/4) (t/((d+1/2)^2 + t^2) - (2(d+1/2)t)/(((d+1/2)^2 + t^2)^2)); \end{aligned}$$

$LB1[d_, a1_, a2_, a3_, t_] := -UB1[d, a1, a2, a3, t];$

**FunctionRange[**

$\{L11[0.722, 1.07, 0.93, 0.365, x] + LB1[0.722, 1.07, 0.93, 0.365, x], x \geq 1\}, x, y]$

(Debug) Out[32]=

$-0.25 < y \leq -0.163523$

Estimates for  $U_{\{2,1\}}(T)$  and  $UB_2(T)$ , which we denote by  $U21$  and  $UB2$  respectively:

(Debug) In[33]:=

$$\begin{aligned} U21[d_, a1_, a2_, a3_, t_] := & (2t/Pi) \log[1 + ((1+2d)/(2t))^2] - \\ & (t/Pi) \log[1 + ((1+4d)/(2t))^2] + (d a1/4) \log[1 + ((1+2d)/(2t))^2] + (4d/Pi) \operatorname{ArcTan}[t/(d+1/2)] - \\ & (4d/Pi) \operatorname{ArcTan}[t/(2d+1/2)] - t/(3Pi ((d+1/2)^2 + t^2)) + t/(6Pi ((2d+1/2)^2 + t^2)) - \\ & (d a1/4) ((d+1/2)/((d+1/2)^2 + t^2) + ((d+1/2)^2 - t^2)/(6((d+1/2)^2 + t^2)^2)) + \\ & (d^2 a2/2) ((d+1/2)/((d+1/2)^2 + t^2) + ((d+1/2)^2 - t^2)/(2((d+1/2)^2 + t^2)^2)) + \\ & (a3/2) (t/((d+1/2)^2 + t^2) - ((d+1/2)t)/(((d+1/2)^2 + t^2)^2)); \end{aligned}$$

$UB2[d_, a1_, a2_, a3_, t_] := (4/Pi) (1/360 + 1/(1022(d+1/2)))/((d+1/2)^2 + t^2)^{(3/2)} +$

$(2/Pi) (1/360 + 1/(1022(2d+1/2)))/((2d+1/2)^2 + t^2)^{(3/2)} + (d a1/2)/$

$(120((d+1/2)^2 + t^2)^{(3/2)} + (d^2 a2/2 + a3/2)(1/6 + 1/(23(d+1/2))))/((d+1/2)^2 + t^2)^{(3/2)};$

**FunctionRange[** $\{U21[0.722, 1.07, 0.93, 0.365, x] + UB2[0.722, 1.07, 0.93, 0.365, x], x \geq 1\}, x, y]$

(Debug) Out[35]=

$0. < y \leq 0.514927$

Estimates for  $L_{\{2,1\}}(T)$  and  $LB2(T)$ , which we denote by  $L21$  and  $LB2$  respectively:

(Debug) In[36]:=

$$\begin{aligned} L21[d_, a1_, a2_, a3_, t_] := & (2t/Pi) \log[1 + ((1+2d)/(2t))^2] - \\ & (t/Pi) \log[1 + ((1+4d)/(2t))^2] - (d a1/4) \log[1 + ((1+2d)/(2t))^2] + (4d/Pi) \operatorname{ArcTan}[t/(d+1/2)] - \\ & (4d/Pi) \operatorname{ArcTan}[t/(2d+1/2)] - t/(3Pi ((d+1/2)^2 + t^2)) + t/(6Pi ((2d+1/2)^2 + t^2)) + \\ & (d a1/4) ((d+1/2)/((d+1/2)^2 + t^2) + ((d+1/2)^2 - t^2)/(6((d+1/2)^2 + t^2)^2)) - \\ & (d^2 a2/2) ((d+1/2)/((d+1/2)^2 + t^2) + ((d+1/2)^2 - t^2)/(2((d+1/2)^2 + t^2)^2)) + \\ & (a3/2) (t/((d+1/2)^2 + t^2) - ((d+1/2)t)/(((d+1/2)^2 + t^2)^2)); \end{aligned}$$

$LB2[d_, a1_, a2_, a3_, t_] := -UB2[d, a1, a2, a3, t];$

**FunctionRange[**

$\{L21[0.722, 1.07, 0.93, 0.365, x] + LB2[0.722, 1.07, 0.93, 0.365, x], x \geq 1\}, x, y]$

(Debug) Out[38]=

$0. < y \leq 0.139901$

Lemma 2.7. We first need to verify equation (2.14). We denote  $f_1(\alpha, \phi)$ ,  $f_2(\alpha, \phi)$ , and  $q_1(\alpha, \phi)$  by  $f1(a_, p_)$ ,  $f2(a_, p_)$ , and  $q1(a_, p_)$  respectively.

(Debug) In[39]:=

```
f1[a_, p_] := (4 / Pi) ArcTan[Sin[p] / (a^(1.222) - Cos[p])] - (2 / Pi) ArcTan[Sin[p] / (a^(1.944) - Cos[p])] +
  (0.722 * 1.07 / 2) Log[a] (1 - a^(1.222) Cos[p]) / (1 - 2 a^(1.222) Cos[p] + a^(2.444));
f2[a_, p_] := (0.722^2 * 0.93 / 2) (Log[a])^2
  (a^(1.222) ((1 + a^(2.444)) Cos[p] - 2 a^(1.222))) / (1 - 2 a^(1.222) Cos[p] + a^(2.444))^2 +
  (0.365 / 2) (Log[a])^2 (a^(1.222) (1 - a^(2.444)) Sin[p]) / (1 - 2 a^(1.222) Cos[p] + a^(2.444))^2;
m12[a_] := FindMaxValue[f1[a, p] + f2[a, p], p];
m2[a_] := FindMaxValue[f2[a, p], p];
Plot[m2[x] - m12[x], {x, 4, Infinity}]
```

(Debug) Out[43]=

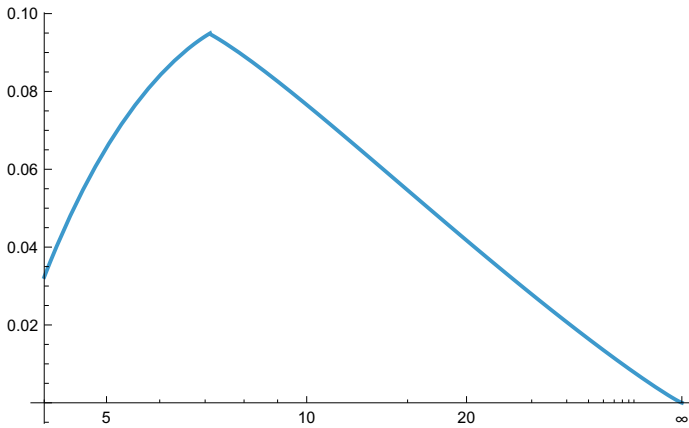

From this examination we conclude equation (2.14). Lastly, the numerical computation of the first 22 terms of the right and side of equation (2.16) yields the following results. The cutoff was chosen to comply with the accuracy tolerance of the FindMaxValue function. Computing more terms should improve the overall result. Although the computations in the last two lines suggest that any improvement is relatively small (probably less than 1).

(Debug) In[44]:=

```
Sum[m12[Prime[n]], {n, 1, 22}]
```

(Debug) Out[44]=

```
1.10834
```

(Debug) In[45]:=

```
0.304 (Zeta'[1.222] / Zeta[1.222] - (Zeta'[1.222] / Zeta[1.222])^2) -
  0.304 Sum[(Log[Prime[n]]^2 Prime[n]^(1.222)) / (1 - Prime[n]^(1.222))^2, {n, 1, 22}]
```

(Debug) Out[45]=

```
4.52428
```

(Debug) In[46]:=

**Sum[m12[Prime[n]], {n, 1, 1 000 000}]**

FindMaxValue: The line search decreased the step size to within the tolerance specified by AccuracyGoal and PrecisionGoal but was unable to find a sufficient increase in the function. You may need more than MachinePrecision digits of working precision to meet these tolerances.

FindMaxValue: The line search decreased the step size to within the tolerance specified by AccuracyGoal and PrecisionGoal but was unable to find a sufficient increase in the function. You may need more than MachinePrecision digits of working precision to meet these tolerances.

FindMaxValue: The line search decreased the step size to within the tolerance specified by AccuracyGoal and PrecisionGoal but was unable to find a sufficient increase in the function. You may need more than MachinePrecision digits of working precision to meet these tolerances.

General: Further output of FindMaxValue::lstol will be suppressed during this calculation.

(Debug) Out[46]=

**4.25777**

(Debug) In[47]:=

**0.304 (Zeta'[1.222]/Zeta[1.222] - (Zeta'[1.222]/Zeta[1.222])^2) -  
0.304 Sum[(Log[Prime[n]]^2 Prime[n]^(1.222))/(1 - Prime[n]^(1.222))^2, {n, 1, 1 000 000}]**

(Debug) Out[47]=

**0.730813**
